# Supplementary material for: Code Representation Learning At Scale
Source: arXiv:2402.01935 source file (2024-02-02)
Supplement: Supplementary file 1 [file dobf_vs_fullmask_appendix.tex]

\begin{figure*}[t]
\centering
\vspace{-10pt}
\begin{subfigure}[b]{0.45\textwidth}
    \centering
% \begin{minted}[fontsize=\tiny,numbersep=2pt, frame=lines, framesep=1mm]{python}
% """Query Code"""
% while 1:
%   n = int(raw_input())
%   if(n==0): break;
%   lisx = map(int, raw_input().split())
%   sum2 = sum(lisx) / (n-1)
%   print sum2
  
% """Top-1 Retrieved Code (Full Mask)"""
% while 1:
%   k = input()
%   if k==0: break
%   print sum(map(int, raw_input().split()))/(k-1)
  
% """Top-1 Retrieved Code (DOBF)"""
% while True:
%   n = int(input())
%   if n==0: break
%   a = [int(input()) for _ in range(n)]
%   a.sort()
%   print(sum(a[1:n-1])//(n-2))
% \end{minted}
\lstset{escapechar=~,style=CustomPy}
\begin{lstlisting}[ 
    basicstyle=\tiny,
]
'''Query Code'''
while 1:
  n = int(raw_input())
  if(n==0): break;
  lisx = map(int, raw_input().split())
  sum2 = sum(lisx) / (n-1)
  print sum2
  
'''Top-1 Retrieved Code (Full Mask)'''
while 1:
  k = input()
  if k==0: break
  print sum(map(int, raw_input().split()))/(k-1)
  
'''Top-1 Retrieved Code (DOBF)'''
while True:
  n = int(input())
  if n==0: break
  a = [int(input()) for _ in range(n)]
  a.sort()
  print(sum(a[1:n-1])//(n-2))
\end{lstlisting}
\caption{Random masking allows the model to leverage syntax beyond identifiers and hence boost the Code2Code search performance, especially when the identifiers do not carry rich semantics. }
\label{fig:code2code_fullm_win}
\end{subfigure}
\hspace{0.5cm}
\begin{subfigure}[b]{0.5\textwidth}
    \centering
% \begin{minted}[fontsize=\tiny,numbersep=2pt, frame=lines, framesep=1mm]{python}
% """NLS Query"""
% # Returns the first row returned for the given query.

% """Top-1 Retrieved Code (Full Mask)"""
% def values(cls):
%   # get all items
%   results = cls.query().fetch()
%   # return list of dictionaries
%   return [result.to_dict() for result in results]
    
% """Top-1 Retrieved Code (DOBF)"""
% def get(self, query, *parameters, **kwparameters):
%   rows = self._query(query, parameters, kwparameters)
%   if not rows:
%     return None
%   elif not isinstance(rows, list):
%     raise MySQLError("Query is not a select query")
%   elif len(rows) > 1:
%     raise MySQLError("Multiple rows returned for 
%         Database.get() query")
%   else:
%     return rows[0]
% \end{minted}
\lstset{escapechar=~,style=CustomPy}
\begin{lstlisting}[ 
    basicstyle=\tiny,
]
'''NLS Query'''
# Returns the first row returned for the given query.

'''Top-1 Retrieved Code (Full Mask)'''
def values(cls):
  # get all items
  results = cls.query().fetch()
  # return list of dictionaries
  return [result.to_dict() for result in results]
    
'''Top-1 Retrieved Code (DOBF)'''
def get(self, query, *parameters, **kwparameters):
  rows = self._query(query, parameters, kwparameters)
  if not rows:
    return None
  elif not isinstance(rows, list):
    raise MySQLError("Query is not a select query")
  elif len(rows) > 1:
    raise MySQLError("Multiple rows returned for 
        Database.get() query")
  else:
    return rows[0]
\end{lstlisting}
\caption{DOBF allows the model to better capture high-level semantics between NL and Code (especially those hidden in identifiers), while random masking suffers and tends to map according to lexical overlap only.}
\label{fig:nl2code_dobf_win}
\end{subfigure}

\vspace{0.5cm}

\begin{subfigure}[b]{0.99\textwidth}
   \centering
    {\normalsize{
        \resizebox{1.0\linewidth}{!} {%
        \begin{tabular}{r c c c c c c c c c c c c}
        \toprule
        & \multicolumn{4}{c}{\oursmall} & \multicolumn{4}{c}{\ourbase} & \multicolumn{4}{c}{\ourlarge} \\
        \cmidrule(lr){2-5} \cmidrule(lr){6-9} \cmidrule(lr){10-13}
        Model 
        & Random & \multirow{2}{*}{DOBF} & Sequ- & Para- 
        & Random & \multirow{2}{*}{DOBF} & Sequ- & Para-  
       & Random & \multirow{2}{*}{DOBF} & Sequ- & Para-  \\ 
        &Mask &  &ential &llel 
        &Mask &  &ential &llel 
        &Mask &  &ential &llel \\
        % \midrule
        \cmidrule(lr){1-1} \cmidrule(lr){2-5} \cmidrule(lr){6-9} \cmidrule(lr){10-13}
        NL2Code &          6.61&  18.51&  23.28& 
                           25.19& 
                           11.26& 22.43&  21.63&  22.91&
                           18.45& -    &   28.66&  29.26\\ 

        Code2Code (In) &   15.58&  13.69&  16.81& 
                           18.46& 
                           26.76&  22.42&  23.86&  27.42&
                           29.15&  -    &  28.69&
                           31.95\\
       
        Code2Code (Cross) & 5.05&  6.11&   7.94&  
                            8.55&
                            15.66&  12.97&  13.27&  17.48&
                            18.77&  -    &  17.38&  22.16\\
       
        Classification  &   71.60&  78.81&  77.61&  
                            75.52&
                            77.78&  83.97&  82.28&  83.05&
                            74.48&  -    &  84.37&  85.74\\
        \bottomrule
        \end{tabular}
        }
    }}
    \caption{DOBF and random masking (Rand Mask) complement each other.  }
\end{subfigure}
    \caption{
     Random Masking (with Full [MASK] tokens) vs. Deobfuscation.}
     \vspace{-4pt}
    \label{tab:dobf_vs_random}
\end{figure*}
