# Supplementary material for: Code Representation Learning At Scale
Source: arXiv:2402.01935 source file (2024-02-02)
Supplement: Supplementary file 2 [file nl2code_examples.tex]

Go
